# Supplementary material for: DebiasGAN: Eliminating Position Bias in News Recommendation with Adversarial Learning
Source: arXiv:2106.06258 source file (2021-06-11)
Supplement: Supplementary file 1 [file supplement.tex]

\section*{Supplementary Materials}

\subsection*{Experimental Environment}

Our experimental environment is built on a Linux server with Ubuntu 16.04 operation system.
The version of Python is 3.6
The server has 4 Tesla V100 GPUs with 32GB memory.
The CPU type is Intel(R) Xeon(R) Platinum 8168 CPU @ 2.70GHz.
The total memory is 128GB.
We use the horovod framework for parallel model training on the 4 GPUs, each of which represents a platform.

\subsection*{Dataset Analysis}

We show the distributions of the displayed positions of news in Fig.~\ref{fig.dis} and the click-through rate (CTR) of news displayed at different positions in Fig.~\ref{fig.ctr}.

\subsection*{Hyperparameter Settings}

The complete hyperparameter settings are listed in Table~\ref{hyper}.
We can see that there are usually fewer news displayed at higher positions and the CTR of news displayed at high positions are usually relatively lower.
Note that since news are not simply sequentially displayed on the webpage, the CTR does not strictly decrease with the increase of positions.

\begin{figure}[!t]
  \centering  
      \includegraphics[width=0.7\linewidth]{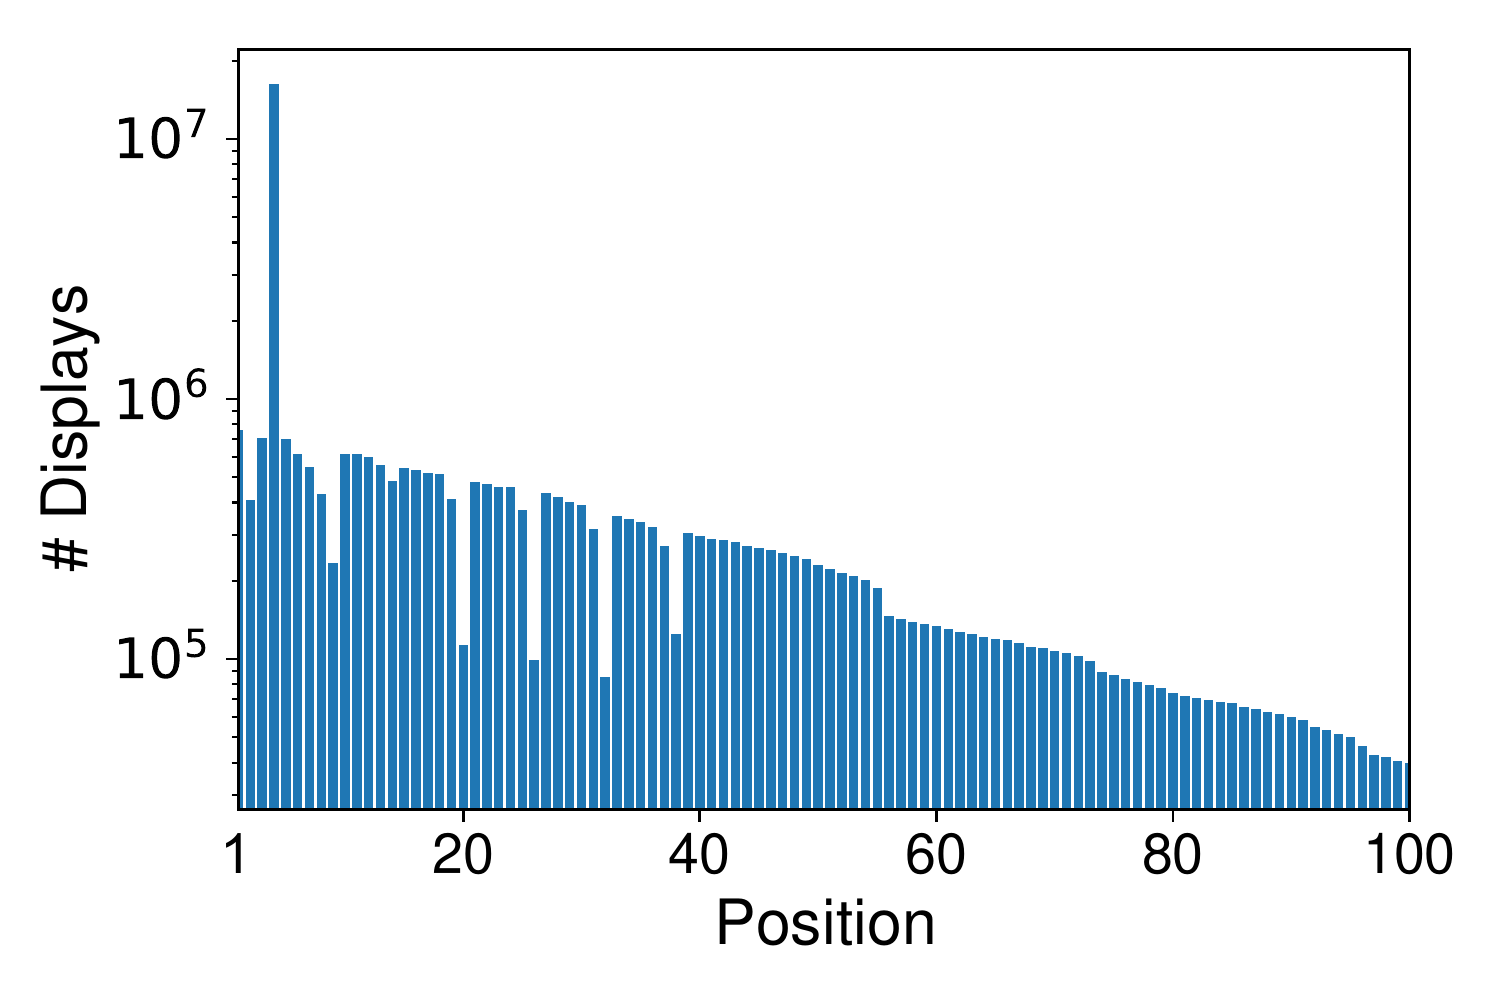} 
 
  \caption{Position distributions in the \textit{News} dataset.}\label{fig.dis}
\end{figure}

\begin{figure}[!t]
  \centering  
      \includegraphics[width=0.7\linewidth]{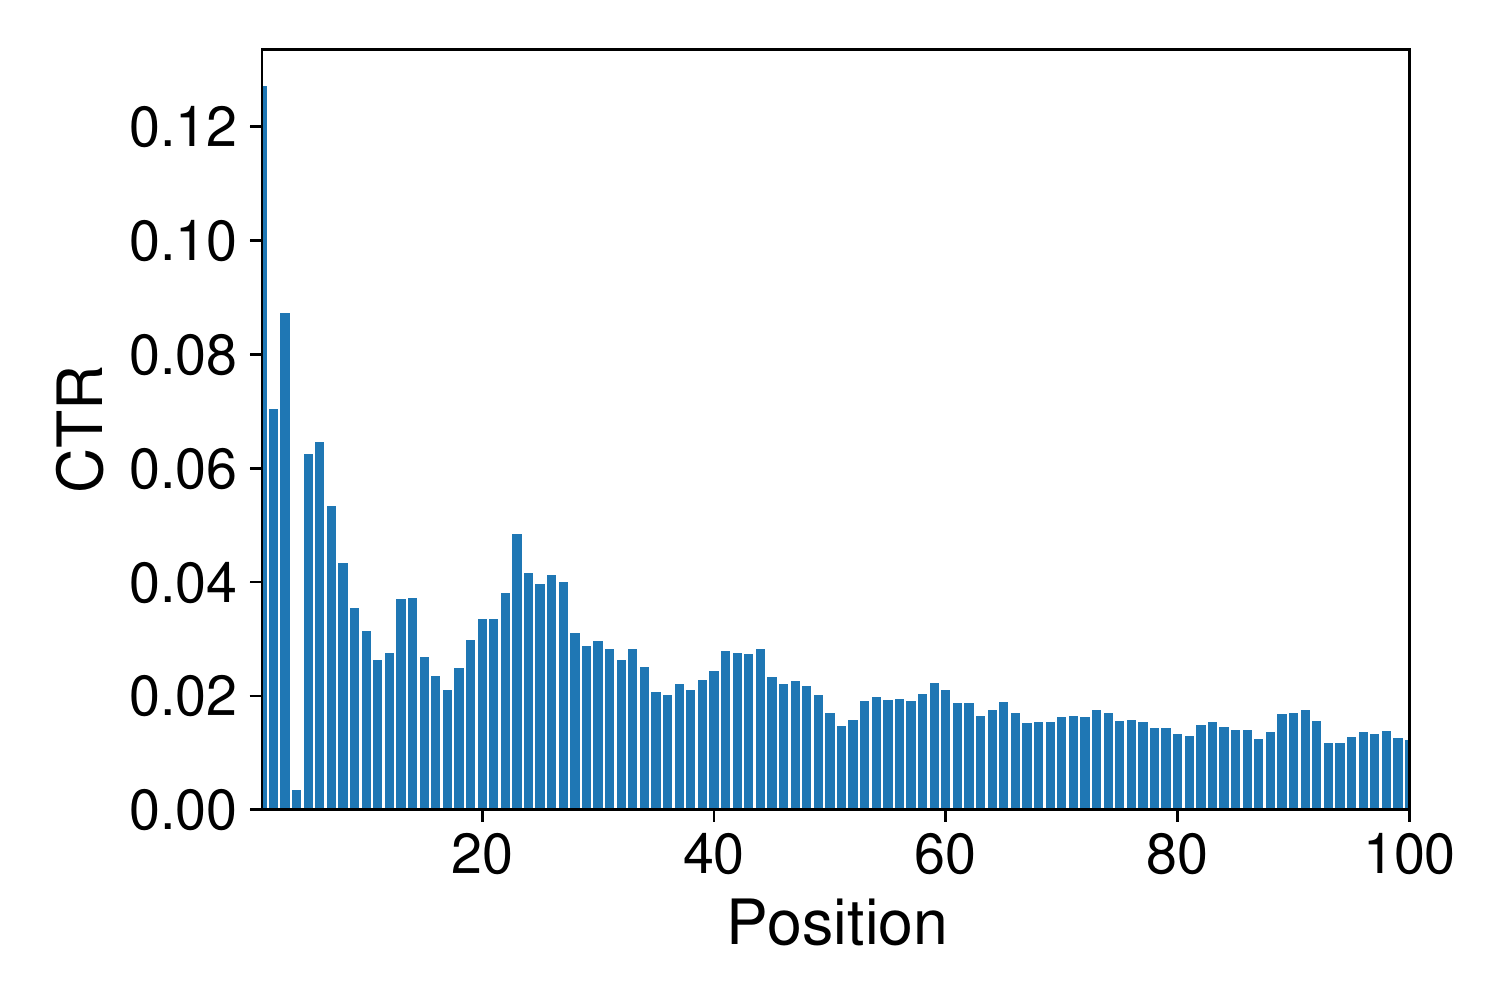} 
 
  \caption{The click-through rate of news displayed at different positions in the \textit{News} dataset.}\label{fig.ctr}
\end{figure}

\begin{table}[h]
\centering
\resizebox{1.0\linewidth}{!}{
\begin{tabular}{l|c}
\hline
\multicolumn{1}{c|}{\textbf{Hyperparameters}}& \textbf{Value}\\ \hline
 embedding dimension                     & 300              \\  
attention head                    & 16      \\ 
head  output size                     & 16      \\ 
Transformer layer                     & 1      \\ 
news title padding length                & 30      \\ 
click history padding length                  & 50      \\ 

$\alpha$                                 & 0.5       \\
dropout                                      & 0.2      \\
optimizer                                    & Adam    \\
learning rate                                 & 1e-4       \\
batch size                                   & 32   \\   
\hline
\end{tabular}
}
\caption{Hyperparameter settings.}\label{hyper}
\end{table}
